# Supplementary material for: Time to Cite: Modeling Citation Networks using the Dynamic Impact Single-Event Embedding Model
Source: arXiv:2403.00032 source file (2024-02-28)
Supplement: Supplementary file 1 [file 6-appendix.tex]

\section{You \emph{can} have an appendix here.}

\newpage
\subsection{Generative Model}

\begin{enumerate}
    \item Input parameters: $\alpha^0, \theta^{0}, \alpha^1, \theta^1, \sigma_{\mathbf{z}}, \sigma_{\mathbf{w}}$
    \item For each node $i \in \mathcal{V}$
    \begin{enumerate}
        \item $t_i \sim Uniform(0,T)$ \hfill Paper appearance times
        \item $\lambda_i^0 \sim Gamma(\alpha^0, \theta^{0})$ \hfill Sample the hyper-parameter for $\kappa_i$
        \item $\kappa_i \sim Poisson(\lambda_i^0)$ \hfill Impact (degree) of the target (cited) papers
        \item $\beta_i \sim Gamma(\alpha^1,\theta^1)$ \hfill Impact of source (citing) papers
        \item $\mathbf{z}_i \sim \mathcal{N}(\bm{0}, \sigma_{\mathbf{z}}^2\mathbf{I})$ \hfill Latent target (cited) paper representations
        \item $\mathbf{w}_j \sim \mathcal{N}(\bm{0}, \sigma_{\mathbf{w}}^2\mathbf{I})$ \hfill Latent source (citing) paper representations
    \end{enumerate}
    \item Relabel nodes $\{1,\ldots,N\}$ such that $t_1\leq t_2 \leq \cdots \leq t_N$
    \item For each node $i \in \mathcal{V}$
    \begin{enumerate}
        \item $\tau_i \sim Gamma(\alpha^1, \theta^1)$ \hfill Sample the precision of log-normal distr.
        \item $\mu_i \sim \mathcal{N}(\alpha^1, 1/{\tau_i})$ \hfill Sample the mean of log-normal distr.
        \item $f_i  \leftarrow \text{ pdf of } LogNormal(\mu_i, 1/{\tau_i})$ \hfill Define the pdf of log-normal distr.
    \end{enumerate}
    \item For each node pair $(i,j)\in\mathcal{V}^2$ where $i<j$
    \begin{enumerate}
        \item $w_{ij} \leftarrow \frac{ \left(\kappa_if_i(t_j-t_i)\right) \beta_j }{ \exp{\left(\|\mathbf{z}_i - \mathbf{w}_j \|\right)} }$
    \end{enumerate}
    \item For each node $i \in \mathcal{V}$
    \begin{enumerate}
        \item $K \leftarrow \min(\kappa_i, N-i)$
        \item $\mathbf{p} \leftarrow (w_{i(i+1)},\ldots,w_{ij},\ldots,w_{iN})/c$ where $c_i := \sum_{k=i+1}^Nw_{ik}$  \hfill Weights of Multi. distr.
        \item $(j_1,\ldots,j_K) \sim Multi_K(N-i,\mathbf{p}, \text{without repl.})$ \hfill Sample $K$ node labels
         \item For each source node $j \in \{j_1+i,\ldots,j_{K}+i\}\subseteq \{i+1,\ldots,N\}$
        \begin{enumerate}
        \item Add link $(j, i)$ \hfill Add a link from $j$ to $i$
        \end{enumerate}
    \end{enumerate}
\end{enumerate}

\begin{table*}[!t]
\caption{AUC-ROC scores for varying representation sizes over three citation networks.}
\label{tab:roc-bip}
\begin{center}
%\resizebox{0.48\textwidth}{!}{%
\begin{tabular}{rcccccccccc}\toprule
\multicolumn{1}{l}{} & \multicolumn{3}{c}{\textsl{ML}} & \multicolumn{3}{c}{\textsl{Phys}} & \multicolumn{3}{c}{\textsl{SoSci}}\\\cmidrule(rl){2-4}\cmidrule(rl){5-7}\cmidrule(rl){8-10}
\multicolumn{1}{r}{Dimension ($D$)}  &1    &2	&3  &1    &2 	&3	 &1    &2  &3 \\\cmidrule(rl){1-1}\cmidrule(rl){2-2}\cmidrule(rl){3-3}\cmidrule(rl){4-4}\cmidrule(rl){5-5}\cmidrule(rl){6-6}\cmidrule(rl){7-7}\cmidrule(rl){8-8}\cmidrule(rl){9-9}\cmidrule(rl){10-10}
\textsc{PAM}    &	\multicolumn{3}{c}{0.810} & \multicolumn{3}{c}{0.838} & \multicolumn{3}{c}{0.796}\\
\textsc{TPAM}    & \multicolumn{3}{c}{0.806} & \multicolumn{3}{c}{0.836} & \multicolumn{3}{c}{0.790}\\
\textsc{Node2Vec}    &-    &0.969	& 0.976 &-    &0.963 	&0.973	 &-    &0.956  & 0.963  \\
\textsc{LDM}         &-    &0.969	& 0.976 &-    &0.963 	&0.973	 &-    &0.956  & 0.963  \\
\midrule
\textsc{\modelabbrev \: Truncated}      &-    &0.968	&0.977  &-    &0.962 	&0.973	 &-    & 0.960  & 0.965  \\
\textsc{\modelabbrev \: Log-Normal}  &-    &0.969	&0.976 & -   &0.961 &0.970 &-    &0.957   &0.964    \\
\bottomrule  
\end{tabular}%
%}
\end{center}
\end{table*}

\subsection{Case-Control Inference}
With \textsc{\modelabbrev} being a distance model, it scales prohibitively as $\mathcal{O}(N^2)$ since the all-pairs distance matrix needs to be calculated. In order to scale the analysis to large-scale networks we adopt an unbiased estimation of the log-likelihood similar to a case-control approach \citep{case_control}. In our formulation, we calculate the log-likelihood as:
 \begin{align}\label{eq:single_event_poisson_likelihood_case_control}
\int_{t_i}^{T}\!\!\!\!CDF(t^{\prime})PDF(t^{\prime}) dt^{\prime}
\end{align}

 \begin{align}\label{eq:single_event_poisson_likelihood_case_control}
\log p_{ij}(\mathcal{G}|\Omega) \!&=\!\!\!\! \sum_{\substack{j: y_{ij}=1}}\! \Big (y_{ij}\log\left(\lambda_{ij}(t_{ij}^*) \right) \nonumber\\ & - \log (1\!+\!\!\int_{t_i}^{T}\!\!\!\!\lambda_{ij}(t^{\prime}) dt^{\prime} ) \Big )\nonumber\\ &+\sum_{j:y_{ij}=0}-\log\left(1\!+\!\!\int_{t_i}^{T}\!\!\!\!\lambda_{ij}(t^{\prime}) dt^{\prime}\right)\nonumber\\ &=l_{1}+l_{0}
\end{align}

Large networks are usually sparse so the link (case) likelihood contribution term $l_{1}$ can be calculated analytically, even for massive networks. The non-link (control) likelihood contribution term $l_{0}$ has a quadratic complexity $\mathcal{O}(N^2)$ in terms of the size of the network, and thus its computation is infeasible. For that, we introduce an unbiased estimator for $l_{i,0}$ which is regarded as a population total statistic \citep{case_control}. We estimate the non-link contribution of a node $\{i\}$ via:
\begin{equation}
    l_{i,0}=\frac{N_{i,0}}{n_{i,0}}\!\!\sum_{k=1}^{n_{i,0}}-\log\left(1\!+\!\!\int_{t_i}^{T}\!\!\!\!\lambda_{ik}(t^{\prime}) dt^{\prime}\right),
\end{equation}
where $N_{i,0}$ is the number of total non-links (controls) for node $\{i\}$, and $n_{i,0}$ is the number of samples to be used for the estimation. We set the number of samples based on the node degrees as $n_{i,0}=5*\text{degree}_i$. This makes inference scalable defining an $\mathcal{O}(cE)$ space and time complexity.

by the \textsc{Truncated} normal distribution:

\begin{align}
f_i(t) = \frac{1}{\sigma}\frac{\phi(\frac{t-\mu}{\sigma})}{\Phi(\frac{\kappa-\mu}{\sigma})-\Phi(\frac{\rho-\mu}{\sigma})}
\end{align}

where $\mu$ and $\sigma$ are the parameters of the distribution which lie in $(\rho,\kappa) \in \mathbb{R}$, $\phi(x)=\frac{1}{\sqrt{2\pi}}\exp{(-\frac{1}{2}x^2)}$, and $\Phi(\cdot)$ is the cumulative distribution function $\Phi(x)=\frac{1}{2}\Big(1+ \text{erf}(\frac{x}{\sqrt{2}})\Big)$.
